# Supplementary material for: Generalized Bayesian Posterior Expectation Distillation for Deep Neural Networks
Source: arXiv:2005.08110 source file (2020-05-16)
Supplement: Supplementary file 2 [file appendix_icml_udl_v1.tex]

\appendix
\section{Additional results on Masked MNIST Data}
Similar to Figure \ref{fig:delta_plot}, we show the trends in distillation performance for convolutional neural networks in Figure \ref{fig:cnn_delta_plot}. The detailed results from the experiments performed using both types of models are given in Table \ref{tab:masked_mnist_results}. Note that the experiments to evaluate the robustness of Bayesian Dark Knowledge for CNNs are performed using the following CNN architecture for both the teacher and the student model: Conv(num\_kernels = 10, kernel\_size = 4, stride = 1) - MaxPool(kernel\_size=2) - Conv(num\_kernels = 20, kernel\_size = 4, stride = 1) - MaxPool(kernel\_size=2) - FC (80) - FC (10). This has also been chosen as the base architecture for experiments performed in Section 4. The hyperparameters are the same as used in Section 3 for fully-connected networks. We observe that the performance trends for distillation as we vary number of training samples and masking rate are very similar for both fully-connected networks and convolutional neural networks. 

To probe deeper into the posterior uncertainty, we present box plots of the posterior predictive distribution on the test set for the teacher model in Figure \ref{fig:boxplot_fcnn}, and Figure \ref{fig:boxplot_cnn} for fully-connected and convolutional  networks respectively. We see that masking has a significant impact on the posterior uncertainty. The entropy results, when complemented with the results in Table \ref{tab:masked_mnist_results} demonstrate that the original Bayesian Dark Knowledge approach is not robust to posterior uncertainty. 

\begin{table}[htbp]
\caption{Distillation performance with different data sizes ($N$), mask sizes ($m$) and masking rates ($r$) using \textbf{fully-connected neural networks}. $\Delta$ denotes the performance gap between teacher and student on test set. Note that the for every row, the test set also has the same masking rate.}
\vspace{0.15in}
\begin{tabular}{cccccc}
\toprule
$N$ & $m$ & $r$ & \begin{tabular}[c]{@{}c@{}}NLL\\ (Teacher)\end{tabular} & \begin{tabular}[c]{@{}c@{}}NLL\\ (Student)\end{tabular} & $\Delta$ \\ \toprule
\multirow{8}{*}{10000} & 0 & 0.000 & 0.138 & 0.173 & 0.036 \\ %\cline{2-6} 
 & 2 & 0.005 & 0.140 & 0.181 & 0.041 \\ %\cline{2-6} 
 & 6 & 0.046 & 0.213 & 0.264 & 0.051 \\ %\cline{2-6} 
 & 10 & 0.128 & 0.314 & 0.392 & 0.078 \\ %\cline{2-6} 
 & 14 & 0.250 & 0.493 & 0.573 & 0.080 \\ %\cline{2-6} 
 & 18 & 0.413 & 0.851 & 0.915 & 0.064 \\ %\cline{2-6} 
 & 22 & 0.617 & 1.600 & 1.634 & 0.034 \\ %\cline{2-6} 
 & 26 & 0.862 & 2.205 & 2.216 & 0.011 \\ \midrule
\multirow{8}{*}{20000} & 0 & 0.000 & 0.090 & 0.121 & 0.031 \\ %\cline{2-6} 
 & 2 & 0.005 & 0.094 & 0.130 & 0.036 \\ %\cline{2-6} 
 & 6 & 0.046 & 0.147 & 0.209 & 0.061 \\ %\cline{2-6} 
 & 10 & 0.128 & 0.228 & 0.334 & 0.106 \\ %\cline{2-6} 
 & 14 & 0.250 & 0.392 & 0.482 & 0.090 \\ %\cline{2-6} 
 & 18 & 0.413 & 0.729 & 0.810 & 0.081 \\ %\cline{2-6} 
 & 22 & 0.617 & 1.550 & 1.600 & 0.050 \\ %\cline{2-6} 
 & 26 & 0.862 & 2.204 & 2.218 & 0.015 \\ \midrule
\multirow{8}{*}{30000} & 0 & 0.000 & 0.071 & 0.093 & 0.022 \\ %\cline{2-6} 
 & 2 & 0.005 & 0.073 & 0.099 & 0.027 \\ %\cline{2-6} 
 & 6 & 0.046 & 0.123 & 0.177 & 0.054 \\ %\cline{2-6} 
 & 10 & 0.128 & 0.195 & 0.269 & 0.074 \\ %\cline{2-6} 
 & 14 & 0.250 & 0.347 & 0.446 & 0.099 \\ %\cline{2-6} 
 & 18 & 0.413 & 0.697 & 0.791 & 0.094 \\ %\cline{2-6} 
 & 22 & 0.617 & 1.524 & 1.584 & 0.059 \\ %\cline{2-6} 
 & 26 & 0.862 & 2.194 & 2.209 & 0.015 \\ \midrule
\multirow{8}{*}{60000} & 0 & 0.000 & 0.052 & 0.080 & 0.027 \\ %\cline{2-6} 
 & 2 & 0.005 & 0.055 & 0.084 & 0.029 \\ %\cline{2-6} 
 & 6 & 0.046 & 0.092 & 0.155 & 0.062 \\ %\cline{2-6} 
 & 10 & 0.128 & 0.159 & 0.246 & 0.087 \\ %\cline{2-6} 
 & 14 & 0.250 & 0.296 & 0.407 & 0.110 \\ %\cline{2-6} 
 & 18 & 0.413 & 0.630 & 0.763 & 0.133 \\ %\cline{2-6} 
 & 22 & 0.617 & 1.495 & 1.565 & 0.070 \\ %\cline{2-6} 
 & 26 & 0.862 & 2.197 & 2.215 & 0.018 \\ \bottomrule
\end{tabular}
\label{tab:masked_mnist_results}
\end{table}
\begin{table}[htbp]
\centering
\caption{Distillation performance with different data sizes ($N$), mask sizes ($m$) and masking rates ($r$) using \textbf{convolutional neural networks}. $\Delta$ denotes the performance gap between teacher and student on test set. Note that the for every row, the test set also has the same masking rate.}
\vspace{0.15in}
\begin{tabular}{cccccc}
\toprule
$N$ & $m$ & $r$ & \begin{tabular}[c]{@{}c@{}}NLL\\ (Teacher)\end{tabular} & \begin{tabular}[c]{@{}c@{}}NLL\\ (Student)\end{tabular} & $\Delta$ \\ \toprule
\multirow{8}{*}{10000} & 0 & 0.000 & 0.138 & 0.173 & 0.036 \\ %\cline{2-6} 
 & 2 & 0.005 & 0.140 & 0.181 & 0.041 \\ %\cline{2-6} 
 & 6 & 0.046 & 0.213 & 0.264 & 0.051 \\ %\cline{2-6} 
 & 10 & 0.128 & 0.314 & 0.392 & 0.078 \\ %\cline{2-6} 
 & 14 & 0.250 & 0.493 & 0.573 & 0.080 \\ %\cline{2-6} 
 & 18 & 0.413 & 0.851 & 0.915 & 0.064 \\ %\cline{2-6} 
 & 22 & 0.617 & 1.600 & 1.634 & 0.034 \\ %\cline{2-6} 
 & 26 & 0.862 & 2.205 & 2.216 & 0.011 \\ \midrule
\multirow{8}{*}{20000} & 0 & 0.000 & 0.090 & 0.121 & 0.031 \\ %\cline{2-6} 
 & 2 & 0.005 & 0.094 & 0.130 & 0.036 \\ %\cline{2-6} 
 & 6 & 0.046 & 0.147 & 0.209 & 0.061 \\ %\cline{2-6} 
 & 10 & 0.128 & 0.228 & 0.334 & 0.106 \\ %\cline{2-6} 
 & 14 & 0.250 & 0.392 & 0.482 & 0.090 \\ %\cline{2-6} 
 & 18 & 0.413 & 0.729 & 0.810 & 0.081 \\ %\cline{2-6} 
 & 22 & 0.617 & 1.550 & 1.600 & 0.050 \\ %\cline{2-6} 
 & 26 & 0.862 & 2.204 & 2.218 & 0.015 \\ \midrule
\multirow{8}{*}{30000} & 0 & 0.000 & 0.071 & 0.093 & 0.022 \\ %\cline{2-6} 
 & 2 & 0.005 & 0.073 & 0.099 & 0.027 \\ %\cline{2-6} 
 & 6 & 0.046 & 0.123 & 0.177 & 0.054 \\ %\cline{2-6} 
 & 10 & 0.128 & 0.195 & 0.269 & 0.074 \\ %\cline{2-6} 
 & 14 & 0.250 & 0.347 & 0.446 & 0.099 \\ %\cline{2-6} 
 & 18 & 0.413 & 0.697 & 0.791 & 0.094 \\ %\cline{2-6} 
 & 22 & 0.617 & 1.524 & 1.584 & 0.059 \\ %\cline{2-6} 
 & 26 & 0.862 & 2.194 & 2.209 & 0.015 \\ \midrule
\multirow{8}{*}{60000} & 0 & 0.000 & 0.052 & 0.080 & 0.027 \\ %\cline{2-6} 
 & 2 & 0.005 & 0.055 & 0.084 & 0.029 \\ %\cline{2-6} 
 & 6 & 0.046 & 0.092 & 0.155 & 0.062 \\ %\cline{2-6} 
 & 10 & 0.128 & 0.159 & 0.246 & 0.087 \\ %\cline{2-6} 
 & 14 & 0.250 & 0.296 & 0.407 & 0.110 \\ %\cline{2-6} 
 & 18 & 0.413 & 0.630 & 0.763 & 0.133 \\ %\cline{2-6} 
 & 22 & 0.617 & 1.495 & 1.565 & 0.070 \\ %\cline{2-6} 
 & 26 & 0.862 & 2.197 & 2.215 & 0.018 \\ \bottomrule
\end{tabular}
\label{tab:cnn-masking_results}
\end{table}
\begin{figure*}[htbp]
    \centering
    \subfigure{\includegraphics[width=0.45\textwidth]{figures/teacher_cnn_nll_missingness_results.pdf}}
    \subfigure{\includegraphics[width=0.45\textwidth]{figures/cnn_missingness_results.pdf}}
    % \caption{(a)  (b) }
    \caption{Left: NLL on the test set using a CNN teacher model. Right: Difference in NLL on the test set between student CNN and teacher CNN.}
    \label{fig:cnn_delta_plot}
\end{figure*}
\begin{figure*}[htbp]
    \centering
    \subfigure[$N=10000$]{\includegraphics[width=0.32\textwidth]{figures/boxplots/teacher_entropy_fcnn_10k.pdf}}
    \subfigure[$N=20000$]{\includegraphics[width=0.32\textwidth]{figures/boxplots/teacher_entropy_fcnn_20k.pdf}}
   % \subfigure[$N=30000$]{\includegraphics[width=0.45\textwidth]{figures/boxplots/teacher_entropy_fcnn_30k.pdf}}
    \subfigure[$N=60000$]{\includegraphics[width=0.32\textwidth]{figures/boxplots/teacher_entropy_fcnn_60k.pdf}}
    % \caption{(a)  (b) }
    \caption{Entropy of the posterior predictive distribution of the teacher model on the test set using \textbf{fully-connected neural networks.}}
    \label{fig:boxplot_fcnn}
\end{figure*}
\begin{figure*}[htbp]
    \centering
    \subfigure[$N=10000$]{\includegraphics[width=0.32\textwidth]{figures/boxplots/teacher_entropy_cnn_10k.pdf}}
    \subfigure[$N=20000$]{\includegraphics[width=0.32\textwidth]{figures/boxplots/teacher_entropy_cnn_20k.pdf}}
    %\subfigure[$N=30000$]{\includegraphics[width=0.45\textwidth]{figures/boxplots/teacher_entropy_cnn_30k.pdf}}
    \subfigure[$N=60000$]{\includegraphics[width=0.32\textwidth]{figures/boxplots/teacher_entropy_cnn_60k.pdf}}
    % \caption{(a)  (b) }
    \caption{Entropy of the posterior predictive distribution of the teacher model on the test set using \textbf{convolutional neural networks.}}
    \label{fig:boxplot_cnn}
\end{figure*}
